# Supplementary material for: Hide Me: Enabling Location Privacy in Heterogeneous Vehicular Networks
Source: arXiv:2001.07170 source file (2020-01-20)
Supplement: Supplementary file 1 [file 7-appendix.tex]

$\mu$ is the set of all resolved privacy levels.
So we have that 
\begin{multline}
    \mu_l (1- p_{\privacy_e,l})^{n_{\privacy_e} - 1 +\sum\limits_{i\in N} n_i} \cdot \prod_{\privacy\in \Privacies\setminus \privacy_e}(1-p_{\privacy,l})^{n_\privacy} = \\
    \mu_1 (1-p_{\privacy_e,1})^{n_{\privacy_e} - 1 + \sum\limits_{i\in N} n_i}   \cdot \prod_{\privacy \in \Privacies\setminus \privacy_e}(1- p_{\privacy,1})^{n_\privacy}
\end{multline}

and 
\begin{multline}
    p_{\privacy_e, l} = 1 - n_{\privacy_e} - 1 + \sum\limits_{i\in N} n_i \sqrt{\frac{\mu_1}{\mu_l} \cdot \prod_{\privacy\in \Privacies\setminus \privacy_e} \left(\frac{1 - p_{\privacy, 1}}{1 - p_{\privacy, l}}\right)^{n_\privacy}} \cdot\\
    (1 - p_{\privacy_e, 1})
\end{multline}

Now

\begin{multline}
    \mu_l\cdot (1- p_{1,l})^{n_{1} - 1 +\sum\limits_{i\in N} n_i} \cdot \prod_{\privacy\in \Privacies\setminus {1,\privacy_e}}(1-p_{\privacy,l})^{n_\privacy} \cdot \\
    \left[ \left(\frac{\mu_1}{\mu_l} \cdot \prod_{\privacy\in \Privacies\setminus \privacy_e} \left(\frac{1 - p_{\privacy, 1}}{1 - p_{\privacy, l}}\right)^{n_\privacy}\right)^{\frac{1}{n_{\privacy_e}-1+\sum\limits_{i\in N}n_i}}\cdot (1 - p_{\privacy,1}) \right]^{n_\privacy} = \\
    \mu_1 (1-p_{\privacy_e,1})^{n_{\privacy_e} - 1 + \sum\limits_{i\in N} n_i}   \cdot \prod_{\privacy \in \Privacies\setminus \privacy_e}(1- p_{\privacy,1})^{n_\privacy}
\end{multline}

So 

\begin{multline}
    \mu_l ^ {\left(1 - \frac{n_{\privacy_e}}{n_\privacy - 1 + \sum\limits_{i \in N} n_i }\right)}  \cdot (1- p_{1,l})^{\left(n_{1} - 1 +\sum\limits_{i\in N} n_i - \frac{n_{\privacy_e} n_1 }{n_\privacy - 1 + \sum\limits_{i \in N} n_i }\right)} \cdot \\
    \prod_{\privacy\in \Privacies\setminus {1,\privacy_e}}(1-p_{\privacy,l})^{\left(n_\privacy - \frac{n_{\privacy} n_{\privacy_e} }{n_{\privacy_e} - 1 + \sum\limits_{i \in N} n_i }\right)} = \\
    \mu_1^{\left(1 - \frac{n_{\privacy_e}}{n_\privacy - 1 + \sum\limits_{i \in N} n_i }\right)} \cdot (1-p_{\privacy_e,1})^{\left(n_{\privacy_e} - 1 + \sum\limits_{i\in N} n_i -  \frac{n_{\privacy_e} n_{1} }{n_{\privacy_e} - 1 + \sum\limits_{i \in N} n_i }\right)}   
\end{multline}

Now 

$$1 - \frac{n_{\privacy_e}}{n_{\privacy_e} - 1 + \sum\limits_{i \in N} n_i } = \frac{\sum\limits_{i \in N}n_i - 1}{n_{\privacy_e} + \sum\limits_{i\in N}n_i - 1}$$

and

$$n_\privacy - \frac{n_{\privacy} n_{\privacy_e} }{n_{\privacy_e} - 1 + \sum\limits_{i \in N} n_i } = \frac{n_{\privacy} \left(\sum\limits_{i\in N}n_i - 1 \right)}{n_{\privacy_e} + \sum\limits_{i\in N}n_i - 1 }$$

So that 
 
\begin{multline}
    \mu_l  \cdot (1- p_{1,l})^{\sum\limits_{i\in N} n_i + n_1 n_{\privacy_e} - 1 } \cdot 
    \prod_{\privacy\in \Privacies\setminus {1,\privacy_e}}(1-p_{\privacy,l})^{n_{\privacy}} = \\
    \mu_1 \cdot (1-p_{\privacy_e,1})^{n_\privacy}   
\end{multline} 
 
% \cdot \\
%     \left[ \left(\frac{\mu_1}{\mu_l} \cdot \prod_{\privacy\in \Privacies\setminus \privacy_e} \left(\frac{1 - p_{\privacy, 1}}{1 - p_{\privacy, l}}\right)^{n_\privacy}\right)^{\frac{1}{n_{\privacy_e}-1+\sum\limits_{i\in N}n_i}}\cdot (1 - p_{\privacy,1}) \right]^{n_\privacy} = \\
%     \mu_1 (1-p_{\privacy_e,1})^{n_{\privacy_e} - 1 + \sum\limits_{i\in N} n_i}   \cdot \prod_{\privacy \in \Privacies\setminus \privacy_e}(1- p_{\privacy,1})^{n_\privacy}
